# Supplementary material for: ePBR: Extended PBR Materials in Image Synthesis
Source: arXiv:2504.17062 source file (2025-04-23)
Supplement: Supplementary file 1 [file X_suppl.tex]

\clearpage
\section{Image composition (Cont')}
\begin{figure*}[h]
    \centering
    \setlength{\resLen}{0.1\linewidth}
    \addtolength{\tabcolsep}{-7pt}
    \begin{tabular}{cccc@{\hskip -2pt}c@{\hskip -2pt}c@{\hskip -2pt}c}
        \begin{overpic}[width=\resLen]{iv/5/normal.png} 
        \end{overpic} &
        \begin{overpic}[width=\resLen]{iv/5/albedo.png} 
        \end{overpic} &
        \begin{overpic}[width=\resLen]{iv/5/roughness.png} 
        \end{overpic} &
        \begin{overpic}[width=\resLen]{iv/5/irradiance.png} 
        \end{overpic} &
        \multirow{2}{*}[28pt]{
            \begin{overpic}[width=2\resLen]{iv/5/im_rgbx.png} 
            \end{overpic}} &
        \multirow{2}{*}[28pt]{
            \begin{overpic}[width=2\resLen]{iv/5/im_ours.png} 
            \end{overpic}} &
        \multirow{2}{*}[28pt]{
            \begin{overpic}[width=2\resLen]{iv/5/im.png} 
            \end{overpic}} \\[-4pt]
        \begin{overpic}[width=\resLen]{iv/5/depth.png} 
        \end{overpic} &
        \begin{overpic}[width=\resLen]{iv/5/metallic.png} 
        \end{overpic} &
        \begin{overpic}[width=\resLen]{iv/5/transparency.png} 
        \end{overpic} &
        \begin{overpic}[width=\resLen]{iv/5/reflect_ssrt.png} 
        \end{overpic}
        \\[-2pt]
        \begin{overpic}[width=\resLen]{iv/6/normal.png} 
        \end{overpic} &
        \begin{overpic}[width=\resLen]{iv/6/albedo.png} 
        \end{overpic} &
        \begin{overpic}[width=\resLen]{iv/6/roughness.png} 
        \end{overpic} &
        \begin{overpic}[width=\resLen]{iv/6/irradiance.png} 
        \end{overpic} &
        \multirow{2}{*}[28pt]{
            \begin{overpic}[width=2\resLen]{iv/6/im_rgbx.png} 
            \end{overpic}} &
        \multirow{2}{*}[28pt]{
            \begin{overpic}[width=2\resLen]{iv/6/im_ours.png} 
            \end{overpic}} &
        \multirow{2}{*}[28pt]{
            \begin{overpic}[width=2\resLen]{iv/6/im.png} 
            \end{overpic}} \\[-4pt]
        \begin{overpic}[width=\resLen]{iv/6/depth.png} 
        \end{overpic} &
        \begin{overpic}[width=\resLen]{iv/6/metallic.png} 
        \end{overpic} &
        \begin{overpic}[width=\resLen]{iv/6/transparency.png} 
        \end{overpic} &
        \begin{overpic}[width=\resLen]{iv/6/reflect_ssrt.png} 
        \end{overpic}
        \\[-2pt]
        \begin{overpic}[width=\resLen]{iv/7/normal.png} 
        \end{overpic} &
        \begin{overpic}[width=\resLen]{iv/7/albedo.png} 
        \end{overpic} &
        \begin{overpic}[width=\resLen]{iv/7/roughness.png} 
        \end{overpic} &
        \begin{overpic}[width=\resLen]{iv/7/irradiance.png} 
        \end{overpic} &
        \multirow{2}{*}[28pt]{
            \begin{overpic}[width=2\resLen]{iv/7/im_rgbx.png} 
            \end{overpic}} &
        \multirow{2}{*}[28pt]{
            \begin{overpic}[width=2\resLen]{iv/7/im_ours.png} 
            \end{overpic}} &
        \multirow{2}{*}[28pt]{
            \begin{overpic}[width=2\resLen]{iv/7/im.png} 
            \end{overpic}} \\[-4pt]
        \begin{overpic}[width=\resLen]{iv/7/depth.png} 
        \end{overpic} &
        \begin{overpic}[width=\resLen]{iv/7/metallic.png} 
        \end{overpic} &
        \begin{overpic}[width=\resLen]{iv/7/transparency.png} 
        \end{overpic} &
        \begin{overpic}[width=\resLen]{iv/7/reflect_ssrt.png} 
        \end{overpic}
        \\[-2pt]
        \begin{overpic}[width=\resLen]{iv/8/normal.png} 
        \end{overpic} &
        \begin{overpic}[width=\resLen]{iv/8/albedo.png} 
        \end{overpic} &
        \begin{overpic}[width=\resLen]{iv/8/roughness.png} 
        \end{overpic} &
        \begin{overpic}[width=\resLen]{iv/8/irradiance.png} 
        \end{overpic} &
        \multirow{2}{*}[28pt]{
            \begin{overpic}[width=2\resLen]{iv/8/im_rgbx.png} 
            \end{overpic}} &
        \multirow{2}{*}[28pt]{
            \begin{overpic}[width=2\resLen]{iv/8/im_ours.png} 
            \end{overpic}} &
        \multirow{2}{*}[28pt]{
            \begin{overpic}[width=2\resLen]{iv/8/im.png} 
            \end{overpic}} \\[-4pt]
        \begin{overpic}[width=\resLen]{iv/8/depth.png} 
        \end{overpic} &
        \begin{overpic}[width=\resLen]{iv/8/metallic.png} 
        \end{overpic} &
        \begin{overpic}[width=\resLen]{iv/8/transparency.png} 
        \end{overpic} &
        \begin{overpic}[width=\resLen]{iv/8/reflect_ssrt.png} 
        \end{overpic}
        \\[-2pt]
        \begin{overpic}[width=\resLen]{iv/9/normal.png} 
        \end{overpic} &
        \begin{overpic}[width=\resLen]{iv/9/albedo.png} 
        \end{overpic} &
        \begin{overpic}[width=\resLen]{iv/9/roughness.png} 
        \end{overpic} &
        \begin{overpic}[width=\resLen]{iv/9/irradiance.png} 
        \end{overpic} &
        \multirow{2}{*}[28pt]{
            \begin{overpic}[width=2\resLen]{iv/9/im_rgbx.png} 
            \end{overpic}} &
        \multirow{2}{*}[28pt]{
            \begin{overpic}[width=2\resLen]{iv/9/im_ours.png} 
            \end{overpic}} &
        \multirow{2}{*}[28pt]{
            \begin{overpic}[width=2\resLen]{iv/9/im.png} 
            \end{overpic}} \\[-4pt]
        \begin{overpic}[width=\resLen]{iv/9/depth.png} 
        \end{overpic} &
        \begin{overpic}[width=\resLen]{iv/9/metallic.png} 
        \end{overpic} &
        \begin{overpic}[width=\resLen]{iv/9/transparency.png} 
        \end{overpic} &
        \begin{overpic}[width=\resLen]{iv/9/reflect_ssrt.png} 
        \end{overpic}
        \\ 
        \multicolumn{4}{c}{Intrinsic representation} & RGB$\leftrightarrow$X & Ours & Reference
    \end{tabular}
    \caption{
        Image composition.
    }
    \label{fig:compose2}
\end{figure*}

\section{Tabulation of specular component integration}

$F$ could be rewritten as,
\begin{equation}
    F(\wh, \wo) = (1 - F_c) \, F_0 + F_c
\end{equation}
where $F_c = (1 - \dotp{\wo}{\whr})^5$
So we can write $\Fs$ in a linear function of $F_0$,
\begin{equation}
    \Fs = A\, F_0 + B
\end{equation}
where
\begin{equation}\begin{aligned}
    A & = \int \frac{1-F_c}{F(\wh, \wo)} \, \fs(\wo, \wi) \, \dotp{\wi}{\n} \intd \wi \\
    B & = \int \frac{F_c}{F(\wh, \wo)} \, \fs(\wo, \wi) \, \dotp{\wi}{\n} \intd \wi
\end{aligned}\end{equation}
combined with Eq~\ref{eqn:microfacet}, we have
\begin{equation}\begin{aligned}
    A & = \int (1-F_c) \, \frac{D(\wh) \, G(\wo, \wi)}{4 \, \dotp{\wo}{\n}} \intd \wi \\
    B & = \int F_c \, \frac{D(\wh) \, G(\wo, \wi)}{4 \, \dotp{\wo}{\n}} \intd \wi
\end{aligned}\end{equation}

We use Monte Carlo simulation with importance sampling to solve the integrations. The pdf used here is,
\begin{equation}
    p(\wh) = \frac{D(\wh) \, \dotp{\n}{\wh}}{4 \, \dotp{\wo}{\wh}}
\end{equation}

So we have,
\begin{equation}\begin{aligned}
    A & \approx \frac{1}{N} \sum_{k=1}^{N} (1-F_c) \, \frac{G(\wo, \wik) \, \dotp{\wo}{\wh_k}}{\dotp{\wo}{\n} \, \dotp{\n}{\wh_k}} \\
    B & \approx \frac{1}{N} \sum_{k=1}^{N} F_c \, \frac{G(\wo, \wik) \, \dotp{\wo}{\wh_k}}{\dotp{\wo}{\n} \, \dotp{\n}{\wh_k}}
\end{aligned}\end{equation}
where $F_c = (1 - \dotp{\wo}{\wh^{(k)}})^5$.
